# Supplementary material for: Magnetic Frustration Enforced Electronic Reconstruction in Ni intercalated NbSe$_{2}$: Suppression of Electronic Orders
Source: arXiv:2511.10160 source file (2025-11-13)
Supplement: Supplementary file 1 [file Suppl_material_BH14936.pdf]

# Supplementary material for

# Magnetic Frustration Enforced Electronic Reconstruction in Ni intercalated $NbSe_2$: Suppression of Electronic Orders

Ashutosh S. Wadge[1*], Alexander Kazakov[1], Xujia Gong[1], Daniel Jastrzebski[1], Bogdan J. Kowalski[2], Artem Lynnyk[2], Lukasz Plucinski[3, 4], Amar Fakhredine[2], Ryszard Diduszko[2], Marta Aleszkiewicz[2], Jedrzej Korczak[1], Dawid Wutke[5], Marcin Rosmus[5], Rafal Kurleto[5], Natalia Olszowska[5], Carmine Autieri[1, 6]† and Andrzej Wisniewski[1, 2]

[1]*International Research Centre MagTop, Institute of Physics, Polish Academy of Sciences, Aleja Lotników 32/46, PL-02668 Warsaw, Poland*
[2]*Institute of Physics, Polish Academy of Sciences, Aleja Lotników 32/46, PL-02668 Warsaw, Poland*
[3]*Peter Grünberg Institut (PGI-6), Forschungszentrum Jülich GmbH, Wilhelm-Johnen-Straße, DE-52428 Jülich, Germany*
[4]*Institute for Experimental Physics II B, RWTH Aachen University, Sommerfeldstraße 14, DE-52074 Aachen, Germany*
[5]*National Synchrotron Radiation Centre SOLARIS Jagiellonian University Czerwone Maki 98, PL-30392 Cracow, Poland*
[6]*SPIN-CNR, UOS Salerno, IT-84084 Fisciano (SA), Italy*

## 1. Material characterization

X-ray diffraction:

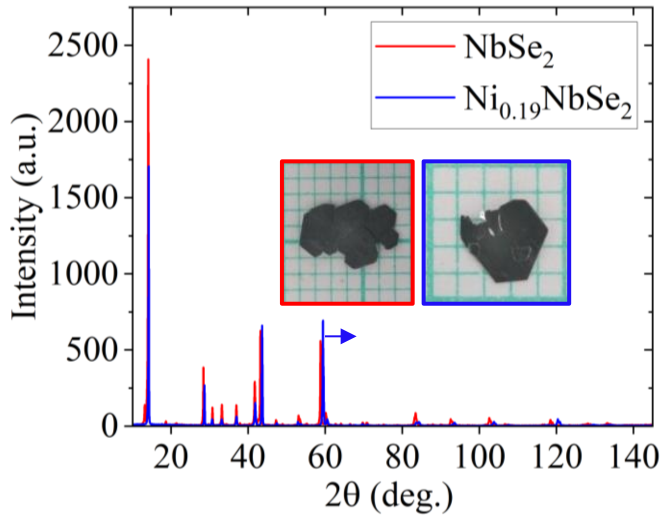


**FIG. S1.** X-ray diffraction (XRD) patterns of pristine $NbSe_2$ and Ni-intercalated $Ni_{0.19}NbSe_2$ showing preferred orientation along the *c*-axis. The primary diffraction peaks remain sharp, indicating good crystallinity in both samples. A slight shift in peak position (highlighted by the arrow) is observed in the doped compound, suggesting lattice modification due to Ni intercalation. Insets show optical images of typical single crystals of pristine $NbSe_2$ and $Ni_{0.19}$ $NbSe_2$ on millimeter-grid paper for scale.

Crystal structure and crystallographic quality of the grown $NbSe_2$ and $Ni_{0.19}NbSe_2$ samples were examined by x-ray powder diffraction using a Rigaku SmartLab 3 kW diffractometer equipped with a Cu anode x-ray tube, operated at 40 kV and 30 mA. The diffraction peaks were verified based on reference data from the Powder Diffraction File PDF-4+2023 RDB database provided by the International Centre for Diffraction Data (ICDD), as shown in **Fig. S1**. The lattice parameters obtained for $NbSe_2$ were $a = b = 3.44445(7)$ Å,. $c = 12.54527(16)$ Å and for $Ni_{0.19}NbSe_2$ $a = b = 3.4550(2)$ Å,. $c = 12.3238(8)$ Å.

Powder X-ray diffraction confirms that the host $NbSe_2$ lattice retains the 2H structure with $NbSe_2$-like lattice constants after Ni intercalation. Within the resolution of our data, we do not observe any superlattice reflections that would indicate long-range 2×2 in-plane ordering of Ni ions. This suggests that, at our composition (x=0.19), Ni atoms are largely disordered within the *ab*-plane. Along the *c*-axis, Ni occupies the octahedral intercalation sites between $NbSe_2$ layers. No additional diffraction peaks consistent with Ni ordering along the c-axis are observed, pointing instead to a statistical occupation of the interlayer sites.

Atomic force microscopy

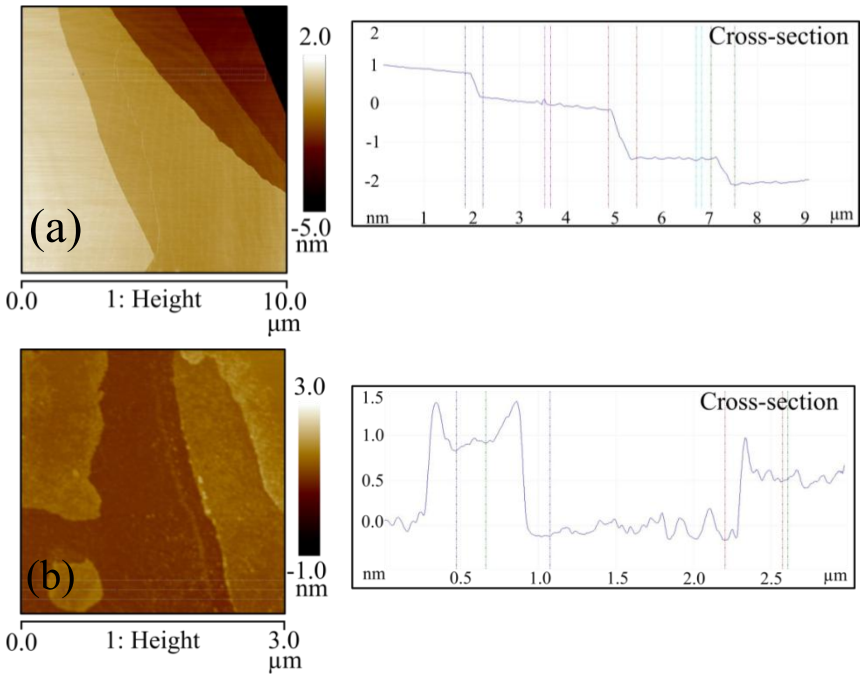


**FIG. S2:** Atomic force microscopy (AFM) images and corresponding cross-sectional height profiles of (a) pristine $NbSe_2$ and (b) $Ni_{0.19}NbSe_2$. The AFM image in (a) shows well-defined terraces with step heights consistent with layered $NbSe_2$, while the cross-sectional plot confirms uniform step heights corresponding to individual layers. In (b), the Ni-intercalated $NbSe_2$ exhibits increased surface roughness and irregular step features, as reflected in the corresponding cross-section, indicating changes in surface morphology due to Ni intercalation.

## 2. Magnetic measurements

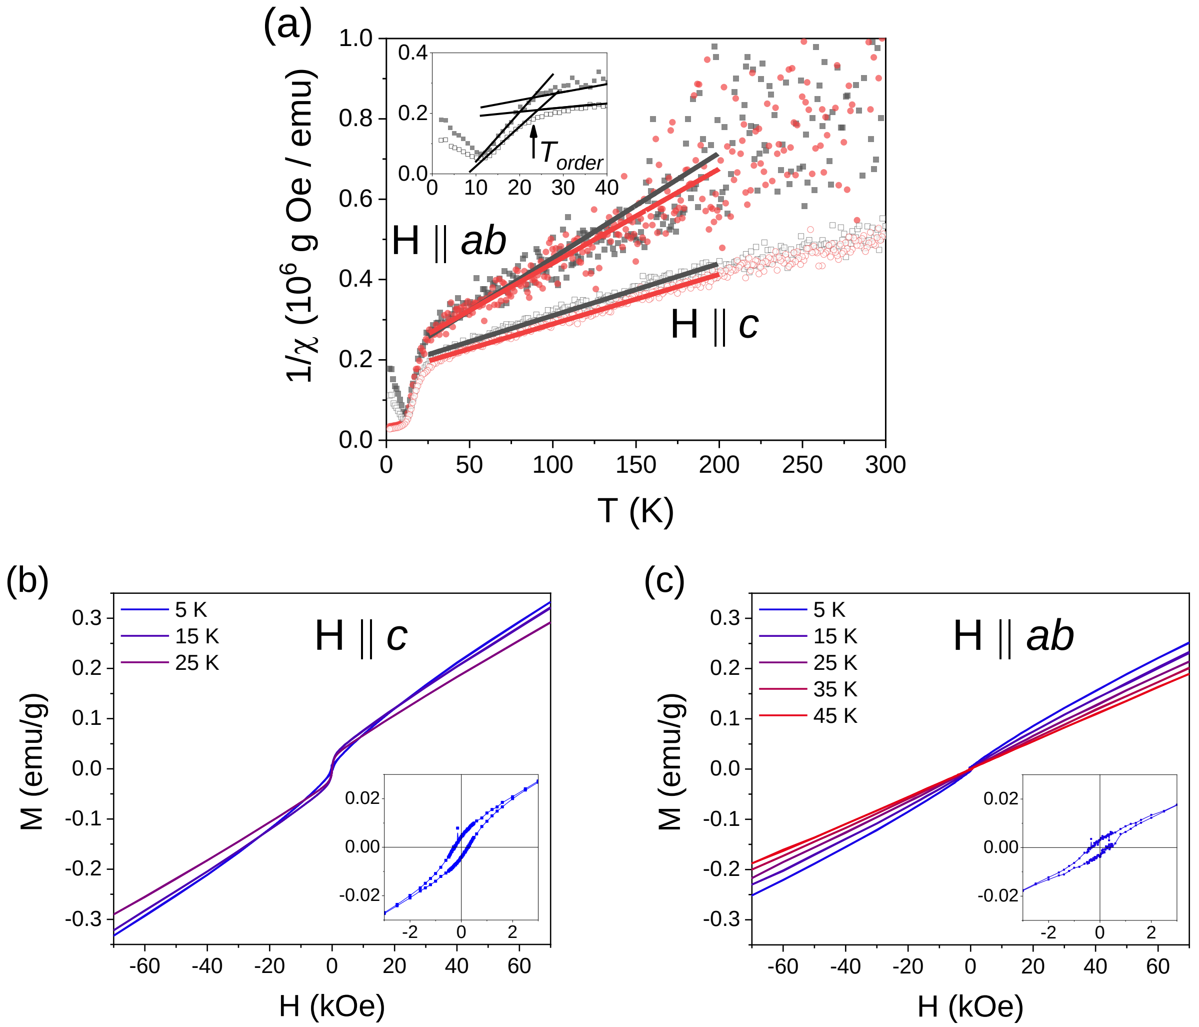


**FIG. S3:** (a) Inverse susceptibility measured in 100 Oe. High temperature data points are fitted with a linear fit according to the Curie-Weiss law. Fitting yields anisotropic Curie-Weiss temperatures $\theta_{CW}$ for two orthogonal field orientations, as described in a main text. Values for $\theta_{CW}$ in the main text are given as an average between ZFC (black points) and FCC (red points) measurement protocols. The magnetic ordering temperature $T_{order}$ was determined as a position of the kink in low temperature part of the curve, as shown in the inset. The given value was taken as an average between all curves. (b,c) Illustration of the temperature evolution of the magnetization loops obtained below and above $T_{order}$.

## 3. ARPES measurements

Fermi surface reconstruction

**Fig. S4** presents a comprehensive comparison of the Fermi surface and low-energy electronic structure of pristine $NbSe_2$ and $Ni_{0.19}NbSe_2$ under different light polarizations, measured using angle-resolved photoemission spectroscopy (ARPES) at photon energy of 64 eV and a temperature of 84 K. Panels (a)

and (b) show the Fermi surfaces acquired with linear and circular polarization. In $Ni_{0.19}NbSe_2$, clear reconstruction features emerge (highlighted by red arrows), including shrunken size of the pocket around $\overline{\Gamma}$ point (shown by Q), indicating the formation of an electron pocket due to Ni intercalation.

Panels (c) and (d) display the corresponding band dispersions along the high-symmetry $\overline{K}$–$\overline{\Gamma}$–$\overline{K}$ direction. A significant increase in spectral intensity near the Fermi level is observed in the intercalated sample, attributed to the emergence of a new electron-like band centered at $\overline{\Gamma}$. This observation is consistent with theoretical predictions of the Fermi surface reconstruction driven by magnetic disorder in a disordered AFM2 phase.

Panels (e) and (f) present band dispersion along the $\overline{M}$–$\overline{\Gamma}$–$\overline{M}$ direction, where two features labeled Δ1 and Δ2 evolve upon intercalation. The entire dataset is repeated across rows for vertical, circular left and circular right polarizations, confirming that the observed spectral changes are robust and polarization-independent. These results underscore the sensitivity of the Fermi surface to Ni intercalation and support the emergence of a magnetically disordered, electronically reconstructed ground state in $Ni_{0.19}NbSe_2$.

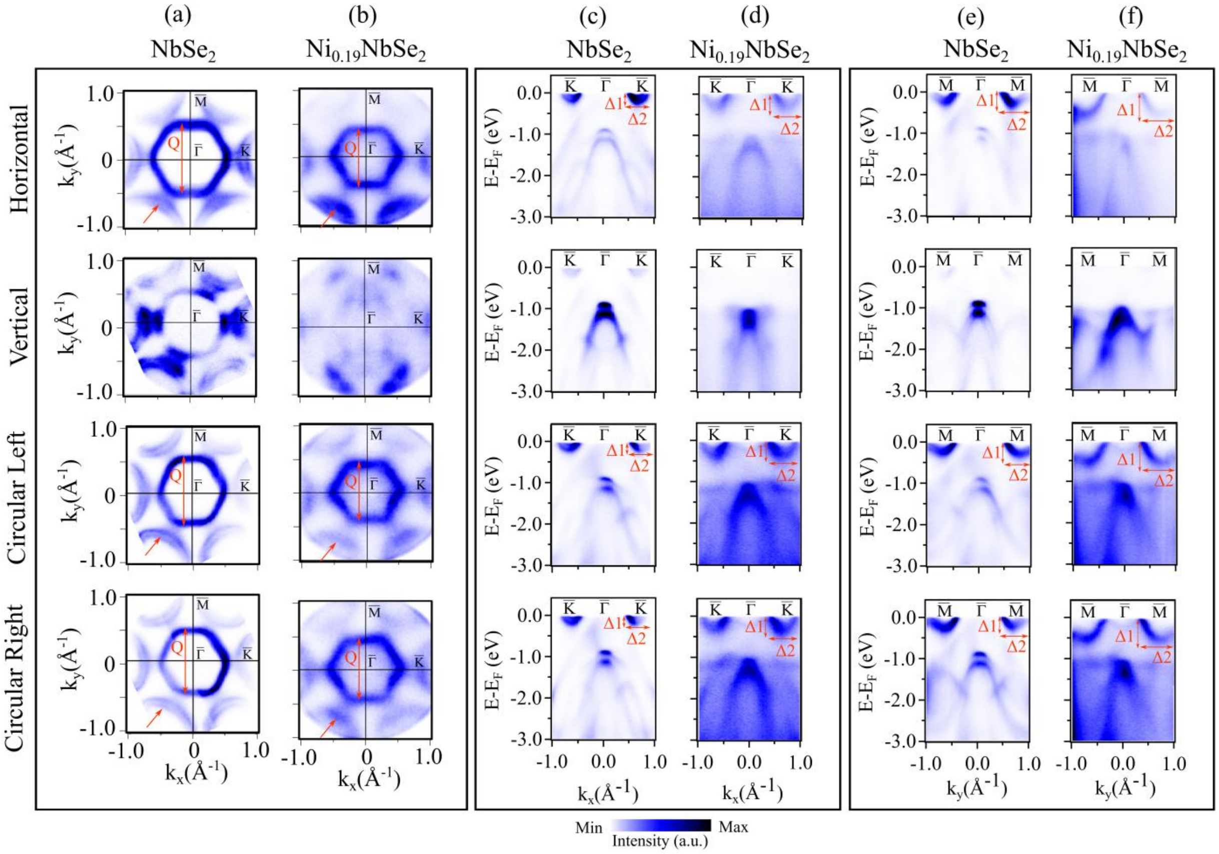


**FIG. S4:** Fermi surface and band structure comparison between pristine $NbSe_2$ and $Ni_{0.19}NbSe_2$ under various light polarizations. (a, b) Fermi surface maps of $NbSe_2$ and $Ni_{0.19}NbSe_2$, respectively, acquired using linear and circular polarization. Red arrows in (a and b) indicate features consistent with the Fermi surface reconstruction upon Ni intercalation. Additionally, Q indicates the size of the Fermi pocket around $\overline{\Gamma}$ which is shrunken after the Ni intercalation (c, d) Corresponding energy–momentum cuts along the $\overline{K}$–$\overline{\Gamma}$–$\overline{K}$ direction under the same polarization show the emergence of an additional electron pocket near the $\overline{\Gamma}$ point in the intercalated sample. (e, f) Energy–momentum cuts along the $\overline{M}$–$\overline{\Gamma}$–$\overline{M}$ path further illustrate the reconstruction features, with Δ1 and Δ2 marking spectral changes. Rows below repeat this comparison using vertical, left circular, and right circular polarization, revealing how polarization selection affects band visibility and symmetry detection. The contrast between pristine and Ni-intercalated $NbSe_2$ demonstrates polarization-sensitive modifications to the Fermi surface and low-energy band structure.

## $k_z$ dispersion

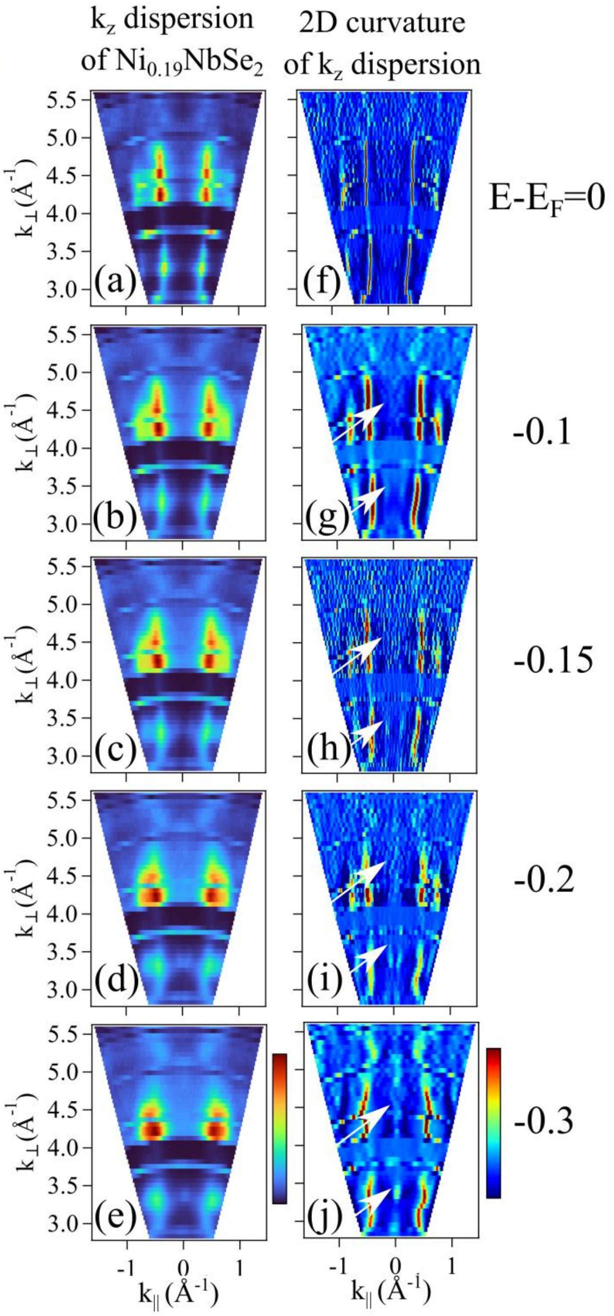


**FIG. S5.** Photon energy dependent $k_z$ dispersions of $Ni_{0.19}NbSe_2$. (a–e) Experimental $k_\parallel$ vs $k_\perp$ intensity maps at constant energies $E-E_F=0, -0.10, -0.15, -0.20, -0.30$ eV. (f–j) Corresponding 2D curvature analysis [1], which enhances weak features and makes the Γ-centered electron pocket more visible (indicated by arrows). The pocket becomes increasingly distinct at binding energies below $E_F$, consistent with its minimum lying at approx. –0.30 eV

Constant energy contour and 3D experimental ARPES:

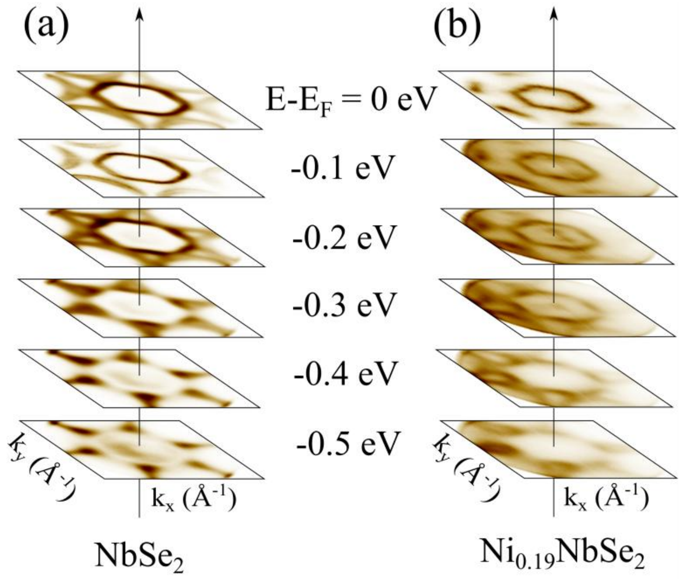


**FIG. S6.** Constant-energy contours of (a) pristine $NbSe_2$ and (b) $Ni_{0.19}NbSe_2$, extracted from ARPES measurements at selected binding energies from $E-E_F=0$ to –0.5 eV. In pristine $NbSe_2$, the Fermi surface consists of hole-like pockets at $\overline{\Gamma}$ and $\overline{K}$ that evolve smoothly with binding energy. In $Ni_{0.19}NbSe_2$, an additional Γ-centered electron pocket emerges below the Fermi level (–0.3 eV and deeper), distinguishing the intercalated compound from the pristine case.

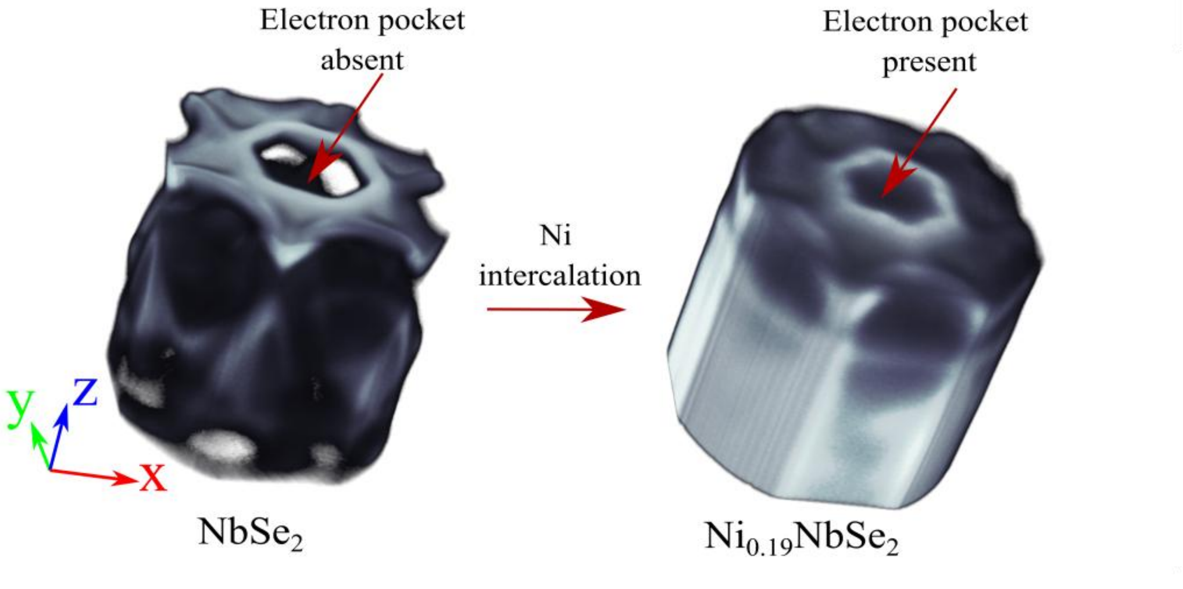


**FIG. S7**. Experimental 3D Fermi-surface volumes reconstructed from ARPES for (left) pristine $NbSe_2$ and (right) $Ni_{0.19}NbSe_2$.

## 4. Orbitally resolved Ni 3d states and hybridization with Nb

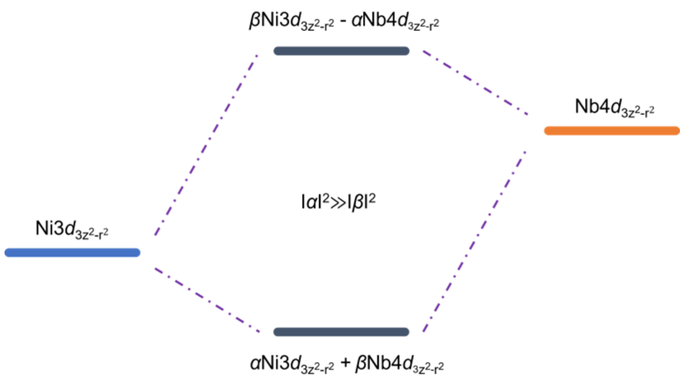


**FIG. S8**. Crystal-field splitting of Ni 3d orbitals in a trigonally distorted octahedron, illustrating the $d_z^2$ orbital hybridization with Nb $d_z^2$

In Ni-intercalated $NbSe_2$, the Ni atoms occupy octahedral sites within a trigonally distorted Se environment. In such an environment, the Ni 3d orbitals are split into $t_{2g}$ and $e_g$ manifolds. In a purely ionic picture, the Ni $d_z^2$ orbital, belonging to the $t_{2g}$ set, would be expected to lie well below the Fermi level.

However, because Ni and Nb atoms are aligned along the crystallographic c-axis, there is strong overlap between Nb $d_z^2$ and Ni $d_z^2$ orbitals. This interaction forms a molecular-orbital–like state, with Nb $d_z^2$ as the dominant component and Ni $d_z^2$ providing a secondary contribution. As a result, states close to the Fermi level carry primarily Nb $d_z^2$ character but are significantly hybridized with Ni $d_z^2$.

**Fig. S8** shows the orbitally resolved density of states for Ni 3d orbitals, illustrating the crystal-field splitting under trigonal distortion as well as the residual $d_z^2$ contribution close to $E_F$. This hybridization highlights the cooperative role of Ni in reshaping the low-energy electronic structure of $Ni_{0.19}NbSe_2$.

## 5. Ni oxidation state and charge transfer

Following the analysis of Gong *et al.* [3], Ni intercalation modifies the charge balance in $Ni_xNbSe_2$. In the ferromagnetic phase the system is half-metallic with a moment of 1 $\mu_B$ per Ni ion, consistent with a nominal $d^9$ configuration ($Ni^{+1}$) and Nb in a $4d^2$ (+3) state. However, a purely ionic picture with $Ni^{2+}$ and $Nb^{4+}$ is not supported. Instead, the effective valence of Ni can be described as $Ni^{2-\delta}$, where $\delta \approx x$ increases with intercalant concentration. At x=0.19, this corresponds to a mixed-valence state between $Ni^{2+}$ and $Ni^{+1}$, implying partial charge transfer to the $NbSe_2$ host. Our own charge analysis at x=1/4 and x=1/3 confirms this approximate scaling.

## 6. Theoretical calculation on the non-magnetic phase of $Ni_{0.19}NbSe_2$

Structural relaxation and supercells

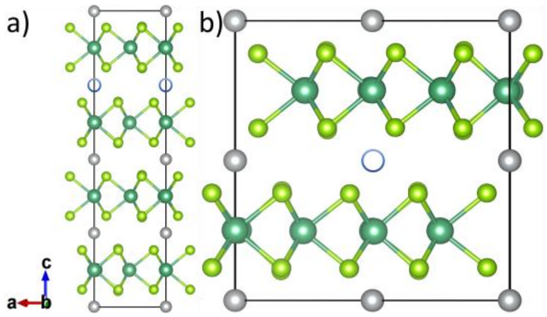


**FIG. S9.** To better approximate the randomness of the defects observed experimentally, we consider two distinct types of Ni-defects by creating supercells expanded along different directions: (a) expansion along the c-axis and (b) in-plane expansion. In the case (a), the system has a hexagonal Brillouin zone, while in (b), the system has an orthorhombic Brillouin zone. In the crystal structure, the location of Ni defects is indicated by unfilled blue circles. Green, lime, and grey balls represent Nb, Se and Ni atoms, respectively.

The experimental lattice constants of pristine $NbSe_2$ were used in the calculations. The position of the magnetic atoms is on top of Nb, as was proposed for $CoNb_4Se_8$ [2]. The position of the Ni atoms is extremely stable and does not change in the presence of atomic defects. We do not consider the possibility of a charge density wave (CDW), since this phenomenon is mainly observed in the low-thickness limit and in undoped systems.

Table S1. Atomic positions of the primitive cell of nonmagnetic structure calculated by DFT+SOC (U=0 eV), WP is the abbreviation for Wyckoff positions.

| Atom | WP | x | y | z |
|---|---|---|---|---|
| Ni | 2*a* | 0 | 0 | 0 |
| Nb(1) | 2*b* | 0 | 0 | 3/4 |
| Nb(2) | 6*h* | 0.01952 | 0.50976 | 3/4 |
| Se(1) | 12*k* | 0.83145 | 0.66290 | 0.88329 |
| Se(2) | 4*f* | 2/3 | 1/3 | 0.39320 |

Electronic Properties

We study the non-magnetic compound $NiNb_4Se_8$, where the unit cell contains two Ni atoms. The results of the structural relaxation are reported in Table S1. We also studied the composition $Ni_{0.19}NbSe_2$ by doubling the unit cell either in-plane or out-of-plane and removing one Ni atom; the resulting stoichiometry is $Ni_{0.19}NbSe_2$. The obtained supercells are shown in **Fig. S9**. In **Fig. S9 (a)**, we present the supercell obtained by expanding along the out-of-plane axis, in which there are three filled layers of Ni atoms and one Ni-empty layer. In contrast, **Fig. S9 (b)** shows the supercell constructed by expanding the cell along the in-plane direction; in this case, there is one filled layer of Ni atoms and one layer partially filled with magnetic atoms. As reported in our previous work [3], Ni intercalation induces magnetism in the stoichiometry $NiNb_4Se_8$. Here, the electronic band structure of non-magnetic $NiNb_4Se_8$ is presented in Fig.S8 as a benchmark for the results on $Ni_{0.19}NbSe_2$. The dispersion is larger in the *ab*-plane, while it is weak along the *c*-axis, although it is stronger than in the pristine compound. Indeed, the Ni atoms produce a bridge between the $NbSe_2$, increasing the band dispersion along the z-axis compared to the pristine van

der Waals systems. In the non-magnetic case, the band structure exhibits a prominent hole pocket at the Γ point similar to that of pristine $NiSe_2$ [4]

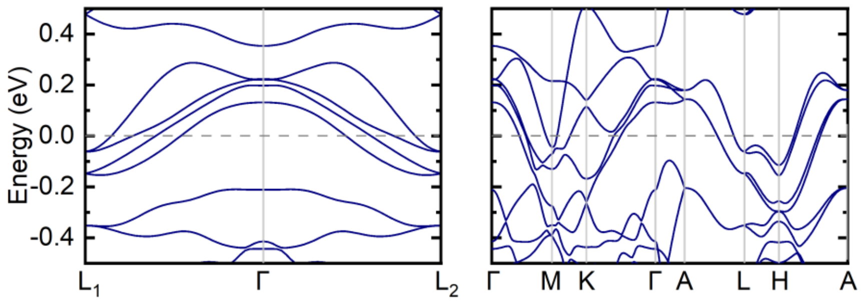


**FIG. S10**. Band structure of the non-magnetic phase of in Ni-intercalated $NbSe_2$ including SOC without Ni vacancy. The left figure displays the results along the high-symmetry path $L_1$-Γ-$L_2$, while the right figure presents the results across all high symmetry points.

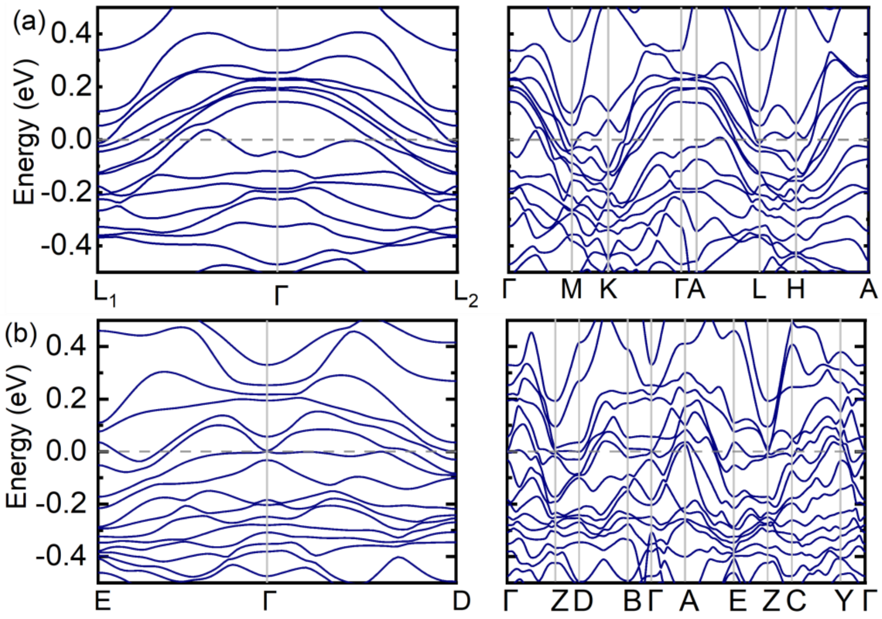


**FIG. S11**. Relativistic band structures of the non-magnetic phase of $Ni_{0.19}NbSe_2$ with two different types of defects: (a) an empty layer of Ni and (b) a half-filled layer of Ni. In the case (a), the system has a hexagonal Brillouin zone, while in the case (b), the system has an orthorhombic Brillouin zone. The left side displays the results around the high-symmetry point Γ while the right side presents the results across all high-symmetry points.

Next, we consider the case with Ni vacancies in the crystal structure to simulate the $Ni_{0.19}NbSe_2$. To investigate the underlying mechanism, we calculate the band structures corresponding to two distinct types of Ni vacancies as shown in **Fig. S11**. By comparing the non-magnetic phase of $Ni_{0.25}NbSe_2$ in **Fig. S10** with nonmagnetic one of $Ni_{0.19}NbSe_2$ in **Fig. S11** (a), it can be observed that most of the bands' dispersions above the Fermi level remain largely unchanged, preserving their prominent hole pockets.

However, the dispersion below the Fermi level becomes corrugated in the vicinity of the Γ point. On the other hand, the situation changes when we have partially filled Ni layers as shown in **Fig. S11 (b)**. In this case, the Ni vacancy induces substantial modifications in the band structure. Notably, none of the bands crossing the Fermi level retain their hole-pocket character. Furthermore, a pronounced electron pocket emerges near the Γ point, which aligns well with the experimental observations. We examined the orbital character of the electron band in the low-energy range at the Γ point. We find that the electron band below the Fermi level is mainly composed of Nb $d_{3z^2-r^2}$ electrons with additional Nb components of $d_{xy}$ and $d_{x^2-y^2}$ states, in addition to the same orbital contribution from Ni atoms, suggesting hybridization. This observation is consistent with the AFM2 phase of $NiNb_4Se_8$ [3]. The two cases reported in Figs. S10 and S11 have different Brillouin zones and cannot be directly compared; however, they provide indications of possible scenarios arising from Ni intercalation

Fermi surface of non-magnetic $Ni_{0.19}NbSe_2$

In **Fig. S12**, we present the Fermi surfaces within the first BZ for $Ni_{0.19}NbSe_2$. The Γ point is centrally located within the BZ, with multiple diagrams illustrating distinct bands for each scenario. The first panel in **Fig. S12 (a)** corresponds to the lowest partially-filled band, which is absent in pristine $NbSe_2$ [5]. The second to the fifth panel exhibits a six-fold Fermi surface nesting pattern. The last panel shows that, in comparison with pristine $NbSe_2$, the peak near the high-symmetry point K disappears, while the peak near the M point remains. For Ni vacancies in the *ab*-plane, due to the specific configuration of the supercell, the characteristic hexagonal BZ of pristine $NbSe_2$ is no longer observed; instead, a parallelepiped-shaped BZ emerges. As illustrated in **Fig. S12 (b)**, six distinct Fermi surfaces can be identified.
sAs shown in **Fig. S12 (b)**, an electron pocket appears in the first panel of the lower set of figures. A magnification of this figure with a shift of 4 meV is reported in **Fig. S13**. According to the band structure calculations, this electron pocket is expected to be quite small, which is consistent with our Fermi surface results. Furthermore, the Fermi surface is no longer nested with the hole pockets but instead forms continuous connections throughout the entire BZ. Even if the results of the last Section cannot be compared directly with the experimental samples, which are in the disordered limit, they give an indication of the level of modification that affects the electronic properties under the influence of intercalated Ni atoms.

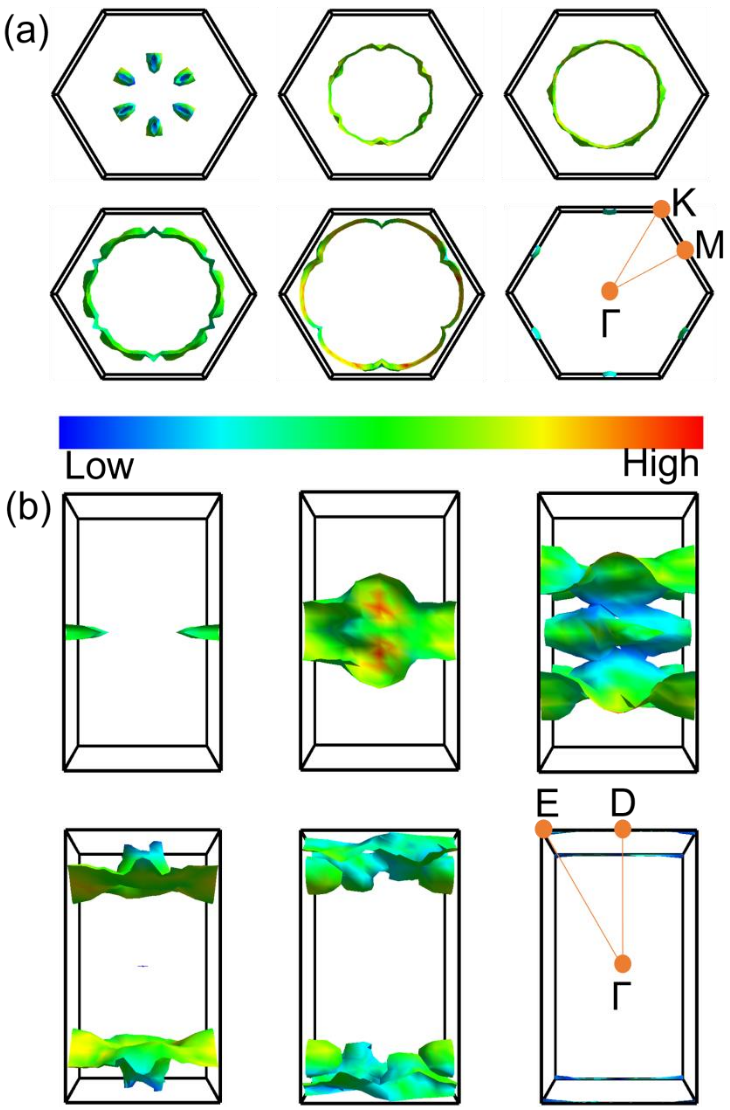


**FIG. S12.** Fermi surface calculated without SOC for the supercell with (a) expansion along the *c*-axis and (b) in the *ab*-plane expansion. When creating a supercell by expanding along the *c*-axis, the Brillouin zone (BZ) retains its hexagonal shape, while by expanding in the *ab*-plane, the BZ adopts parallelepiped geometry. A top-down view, complemented by a perspective image, depicts the Fermi surface. The colormap represents the Fermi velocity. We plot the high-symmetry points of the hexagonal shape of the $k_z = 0$ plane along Γ-K-M in the last panel of (a), and the high-symmetry points of the high-symmetry points along Γ-E-D, where E and D lie in the $k_z = 0.5$ plane along Γ-E-D, where E and D lie in the $k_z = 0.5$ plane in the last panel of (b).

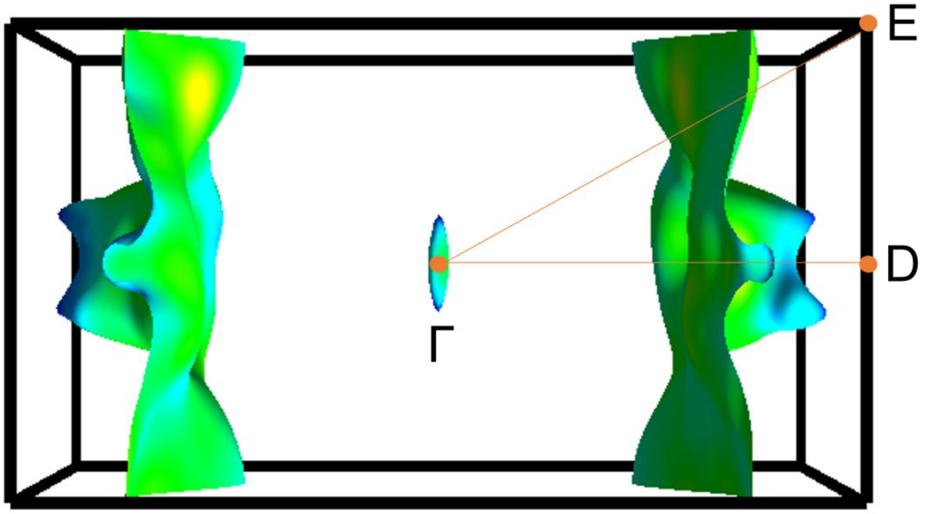


**FIG. S13.** Fermi surface calculated for a supercell with partially filled Ni atoms and a shift of 4 meV of the Fermi surface. We observe an electron pocket at the Γ point. We plot the high-symmetry points of parallelepiped geometry along Γ-E-D, where E and D lie in the $k_z$ = 0.5 plane

## References


[1] P. Zhang, P. Richard, T. Qian, Y. M. Xu, X. Dai, and H. Ding, Review of Scientific Instruments **82**, 043712 (2011).

[2] R. B. Regmi, H. Bhandari, B. Thapa, Y. Hao, N. Sharma, J. McKenzie, X. Chen, A. Nayak, M. El Gazzah, B. G. Markus, et al., Nature Communications **16**, 4399 (2025).

[3] X. Gong, A. Fakhredine, and C. Autieri, Phys. Rev. B 112, 184401 (2025).

[4] K. Rossnagel, O. Seifarth, L. Kipp, M. Skibowski, D. Vos, P. Krüger, A. Mazur, and J. Pollmann, Physical Review B **64**, 235119 (2001).

[5] M. Johannes, I. Mazin, and C. Howells, Physical Review B **73**, 205102 (2006).
